# Supplementary material for: Offline Reinforcement Learning for LLM Multi-Step Reasoning
Source: arXiv:2412.16145 source file (2024-12-25)
Supplement: Supplementary file 1 [file appendix.tex]

\section{Connection and Difference to Direct Reward Optimization}
